# Supplementary material for: AutoShot: A Short Video Dataset and State-of-the-Art Shot Boundary Detection
Source: arXiv:2304.06116 source file (2023-04-12)
Supplement: Supplementary file 1 [file supple.tex]

% CVPR 2023 Paper Template
% based on the CVPR template provided by Ming-Ming Cheng (https://github.com/MCG-NKU/CVPR_Template)
% modified and extended by Stefan Roth (stefan.roth@NOSPAMtu-darmstadt.de)

\documentclass[10pt,twocolumn,letterpaper]{article}

%%%%%%%%% PAPER TYPE  - PLEASE UPDATE FOR FINAL VERSION
% \usepackage[review]{cvpr}      % To produce the REVIEW version
\usepackage{cvpr}              % To produce the CAMERA-READY version
%\usepackage[pagenumbers]{cvpr} % To force page numbers, e.g. for an arXiv version

% Include other packages here, before hyperref.
\usepackage{graphicx}
\usepackage{amsmath}
\usepackage{amssymb}
\usepackage{booktabs}
\usepackage{bm}
\usepackage[accsupp]{axessibility}  % Improves PDF readability for those with disabilities.

% It is strongly recommended to use hyperref, especially for the review version.
% hyperref with option pagebackref eases the reviewers' job.
% Please disable hyperref *only* if you encounter grave issues, e.g. with the
% file validation for the camera-ready version.
%
% If you comment hyperref and then uncomment it, you should delete
% ReviewTempalte.aux before re-running LaTeX.
% (Or just hit 'q' on the first LaTeX run, let it finish, and you
%  should be clear).
\usepackage[pagebackref,breaklinks,colorlinks]{hyperref}

\usepackage{amsfonts}
\usepackage{pifont}% http://ctan.org/pkg/pifont
\newcommand{\cmark}{\ding{51}}%
\newcommand{\xmark}{\ding{55}}%

% Support for easy cross-referencing
\usepackage[capitalize]{cleveref}
\crefname{section}{Sec.}{Secs.}
\Crefname{section}{Section}{Sections}
\Crefname{table}{Table}{Tables}
\crefname{table}{Tab.}{Tabs.}

%%%%%%%%% PAPER ID  - PLEASE UPDATE
 % *** Enter the CVPR Paper ID here

\begin{document}

% Yufang Huang$^3$,
% \quad $^3$Cornell University
%%%%%%%%% TITLE - PLEASE UPDATE
\title{AutoShot: A Short Video Dataset and State-of-the-Art Shot Boundary Detection}
\author{Wentao Zhu$^1$, Yufang Huang$^3$, Xiufeng Xie$^1$, Wenxian Liu$^1$, \\ Jincan Deng$^1$, Debing Zhang$^1$, Zhangyang Wang$^2$, Ji Liu$^1$ \\
$^1$Kuaishou Technology \quad $^2$University of Texas at Austin \quad $^3$Cornell University}

% \def\@name{ \emph{Wentao Zhu*\thanks{*Equal contributions. https://github.com/wentaozhu/speechnas.git}, Tianlong Kong*, Shun Lu, Jixiang Li,},  \\ \emph{Dawei Zhang, Feng Deng, Xiaorui Wang, Sen Yang, Ji Liu}}

% \address{Kuaishou Technology}

% \author{First Author\\
% Institution1\\
% Institution1 address\\
% {\tt\small firstauthor@i1.org}
% % For a paper whose authors are all at the same institution,
% % omit the following lines up until the closing ``}''.
% % Additional authors and addresses can be added with ``\and'',
% % just like the second author.
% % To save space, use either the email address or home page, not both
% \and
% Second Author\\
% Institution2\\
% First line of institution2 address\\
% {\tt\small secondauthor@i2.org}
% }
\maketitle

%%%%%%%%% ABSTRACT
\section{SHOT Dataset}
To accelerate the study of short video related shot boundary detection, we collect 853 short videos from one of the most widely used short video platforms. The dataset property comparison is listed in Table~\ref{tab:dataset}. The total number of frames is 960,794, close to one million frames. The frame-wise shot boundary annotation is a heavy task. %To alleviate the burden of laborious annotation, we develop two kinds of annotation platforms, coarse to fine frame-wise annotation and video thumbnail image based annotation. 

% The coarse to fine frame-wise annotation consists of two stage annotations. In the first stage annotation, we firstly extract frames with a down-sampling rate of ten. Then we conduct the annotation based on frames in the down-sampled video. To obtain the frame-wise annotation, we back-trace the transition from the original video, and extract the nearby 40 frames. In the second stage annotation, we obtain the final accurate shot transition based on the back-traced frames. The coarse to fine two stage annotation significantly reduces the workload. However, we find that the missing rate is too high, probably because 1) the large numbers of short videos have shot length less than ten as shown in the right of Fig.~\ref{fig:len_compare}, and 2) the annotating based on the down-sampled video cannot clearly and accurately identify small inter-shot changes,~\textit{e.g.}, the gradual transitions.

Inspired by the frame processing in TransNetV2~\cite{souvcek2020transnet}, we develop a video thumbnail image based annotation by resizing each frame to be 48$\times$27 as shown in Fig.~\ref{fig:video_thumbnail}. The frame number is adaptively displayed in the upper left corner of each frame, which significantly reduces the annotator's efforts for frame number check. If the pixel value is dark in the frame number position, we display the frame number in light color. Otherwise, we display the frame number in dark color. We have three experts and an annotation team to complete all the annotation of 960,794 frames. The annotation team conducts the annotation for 459 short videos and obtains 6,111 shots totally. After the annotation, we conduct an expert inspection for the 6,111 annotations. We randomly choose 200 shot annotations, and find that 2\% error rate for the 6,111 shot annotations exists. Considering the ambiguity of the shot definition and the annotation difference of annotators, we believe that the 2\% error rate of the 6,111 shots is acceptable.

The quality of annotations on the test set directly affects the accurate evaluation of benchmark methods,~\textit{i.e.}, the quality of the short video dataset. To guarantee the high quality of the shot boundary annotations on the test set, we randomly choose 200 short videos from the rest of 394 short videos annotated by the three experts as the test set. The expert team is the production team who defines the shot transitions and writes the annotation guideline. Then the guideline and data are sent to contractors for the annotation using the thumbnail images, and QA auditing is conducted by the production team. Because of the importance of the test set, it is labeled by the production team completely. For the 200 test short videos, we employ two round annotations, where the first round yields 2,616 shots. In the second round, we conduct a rigorous check for the annotations. In addition to fixing a handful of false positive annotations, which cannot be corrected by our manually designed rules for the automated inspection, the second round totally yields 2,716 shots,~\textit{i.e.}, re-collecting 100 shots from false negatives.  % overall.  leveraging the predictions of TransNetV2~\citep{souvcek2020transnet} and other two model checkpoints of our AutoShot
\begin{figure}[t]
  \centering
  \includegraphics[trim={0 10cm 18cm 0},clip,width=\linewidth]{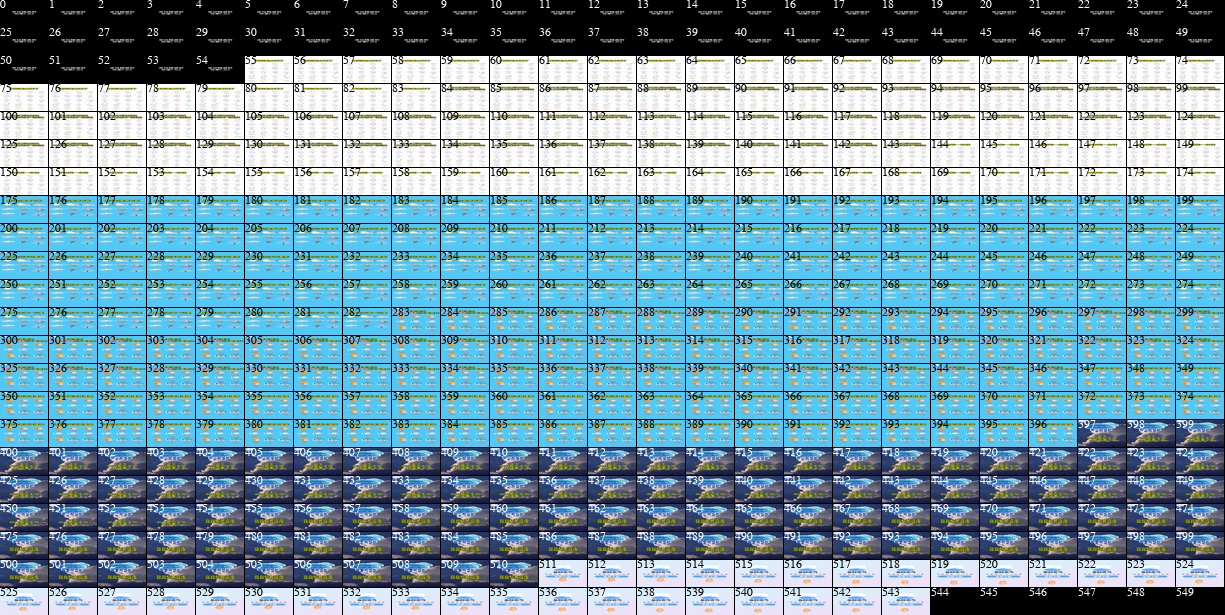}
   \caption{A thumbnail image for one case from our collected SHOT dataset. The frame number is displayed in the upper left corner of each frame.}  % The video thumbnail image clearly demonstrates shot transitions, which greatly reduces the annotation labor and is a useful tool for high quality shot boundary annotation.
   \label{fig:video_thumbnail}
\end{figure}

\begin{table}
  \centering
  \begin{tabular}{@{}lcccc@{}}
    \toprule
    Dataset  & BBC & RAI & ClipShots & SHOT  \\
    \midrule
    % Gradual Trans. &\xmark &\xmark &\cmark &\cmark  \\
    \begin{tabular}{@{}l@{}}Complex Gradual Trans.\end{tabular} &\xmark &\xmark &\xmark &\cmark  \\
    % Large Motion &\xmark &\xmark &\cmark &\cmark  \\
    Virtual Scene &\xmark &\xmark &\xmark &\cmark  \\
    Ternary Video &\xmark &\xmark &\xmark &\cmark  \\
    Avg. Video Len. (s) & 2944.8 & 590.5 &236.5 & 39.5\\
    Avg. Shot Len. (s) & 6.57 & 5.65 &15.34 &2.59 \\
    \bottomrule
  \end{tabular}
  \caption{Comparison of different short boundary detection datasets.}  %   Our SHOT differs significantly from previous datasets.
  \label{tab:dataset}
\end{table}

In the dataset, for each short video, we have a text file with the same name as the video consisting of the annotations of the shot boundaries,~\ie, the beginning and the end frame number of each shot per line, as shown in the following Fig.~\ref{fig:text_supervision}. If there is no gradual transition, as in most shots, the beginning frame number of the next shot should be the next frame number of the end frame number of the current shot. For instance, the end frame number of the first shot is 72, and the beginning frame number of the second shot is 73. If there is a gradual transition, the beginning frame number is a clear transition, and the gap between the end frame number of the last shot and the beginning frame number of the current shot is the gradual transition. For instance, the shot in line 2 ends with frame number 102 as shown in Fig.~\ref{fig:text_supervision}, and the shot in line 3 begins with frame number 109. The frames between 102 and 108 are gradual transitions, as shown in the yellow circle of Fig.~\ref{fig:vis_supple}. Fig.~\ref{fig:vis_supple} is a thumbnail image for one whole video same as Fig.~\ref{fig:text_supervision}, and the light, red and pink colors mark the ground truth shot boundary annotation.

\begin{figure}[t]
  \centering
  \includegraphics[width=0.7\linewidth]{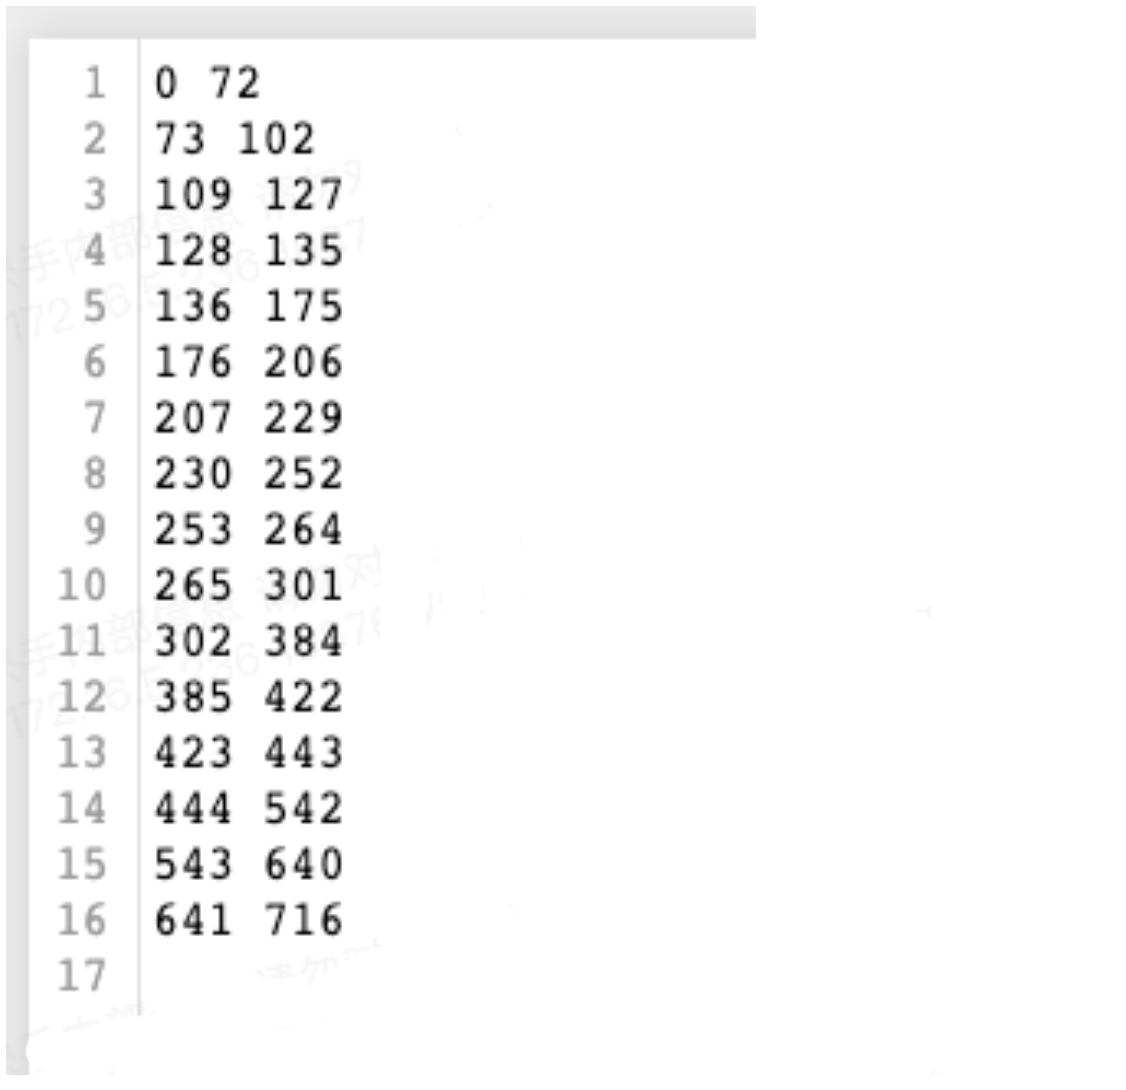}
   \caption{The shot boundary annotation text file. Each line denotes the beginning and the end frame number of one shot.}  % The video thumbnail image clearly demonstrates shot transitions, which greatly reduces the annotation labor and is a useful tool for high quality shot boundary annotation.
   \label{fig:text_supervision}
\end{figure}
\begin{figure}[t]
  \centering
  \includegraphics[width=\linewidth]{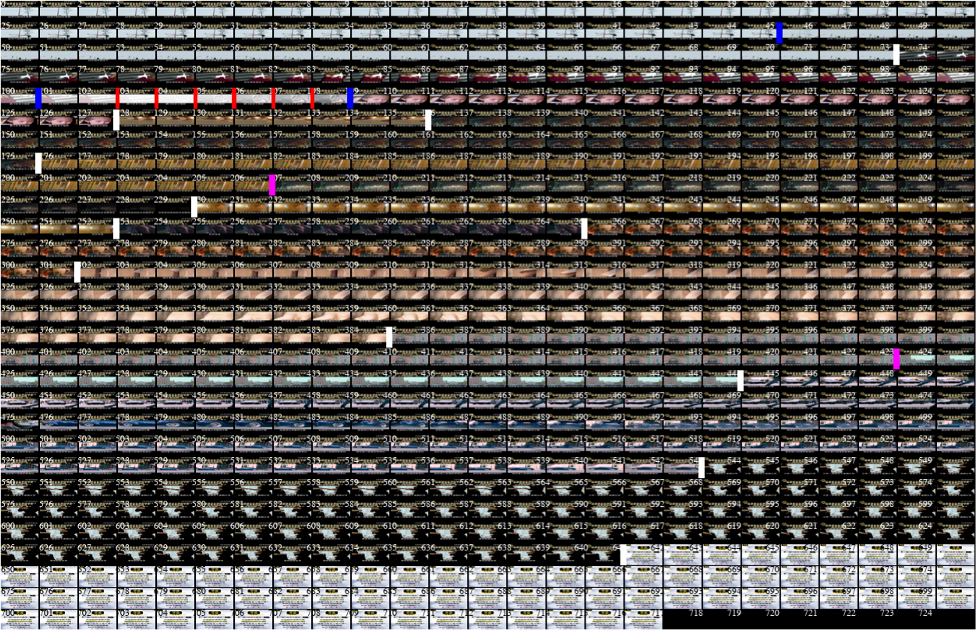}
   \caption{A thumbnail image for the same video as Figure~\ref{fig:text_supervision}. Light, red and pink colors mark the ground truth shot boundary annotation. The yellow circle denotes one gradual transition from frame 102 to frame 108.}  % The video thumbnail image clearly demonstrates shot transitions, which greatly reduces the annotation labor and is a useful tool for high quality shot boundary annotation.
   \label{fig:vis_supple}
\end{figure}

To evaluate the shot boundary detection fairly, we follow the evaluation of ClipShots dataset in~\cite{souvcek2020transnet}. If the detected end frame number is within two frames of the annotation, the detected boundary is a true positive. For a gradual transition, if the detected end frame number is within the gradual transition, it is also a true positive. The metric evaluation script can be found in~\url{ https://github.com/soCzech/TransNetV2/blob/master/training/metrics_utils.py#L26}.

\section{More Visual Comparison Results}
We add more figures in the supplementary to compare the prediction of AutoShot (blue, light, pink, cyan), TransNetV2~\cite{souvcek2020transnet} (green, yellow, light, cyan) and ground truth (red, light, pink, yellow) in Fig.~\ref{fig:pred_supp}. The light color shows that both TransNetV2 and AutoShot have true positive on that frame, as shown in the video thumbnail image of Fig.~\ref{fig:pred_supp} (a). The blue cuts in the Fig.~\ref{fig:pred_supp} (b) show AutoShot successfully detects (within two frames of ground truth) minor shot transitions in the middle of the video. Fig.~\ref{fig:pred_supp} (c) is a vertically ternary structured video, where the scene changes slightly and the minor shot transition is quite difficult to detect. The pink cut in Fig.~\ref{fig:pred_supp} (d) shows AutoShot detects the shot transition, while the TransNetV2 fails. The blue color in frame one of Fig.~\ref{fig:pred_supp} (d) shows AutoShot has a false positive detection, and it is visually reasonable that there is a gradual transition at the beginning of the video.

\begin{figure}[t]
  \centering
  (a)
  \includegraphics[width=0.95\linewidth]{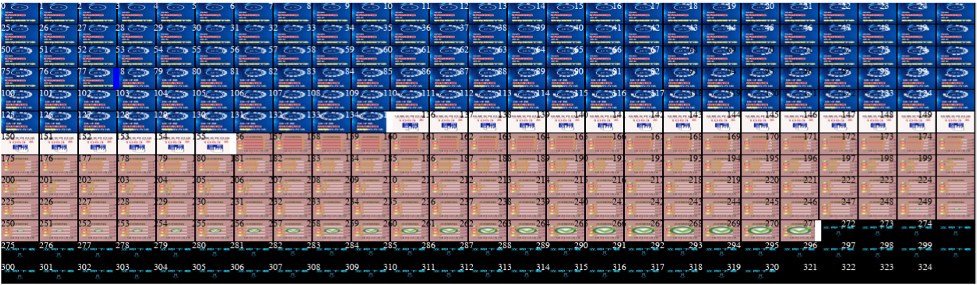}
  (b)
  \includegraphics[width=0.95\linewidth]{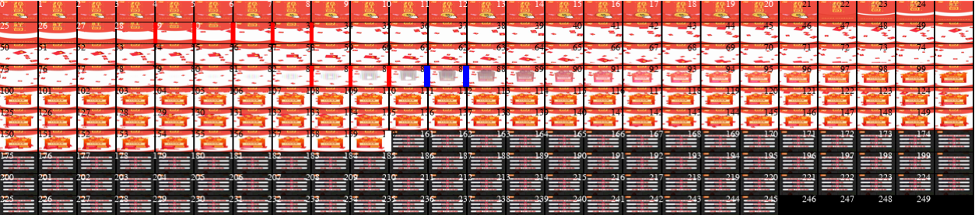}
  (c)
  \includegraphics[width=0.95\linewidth]{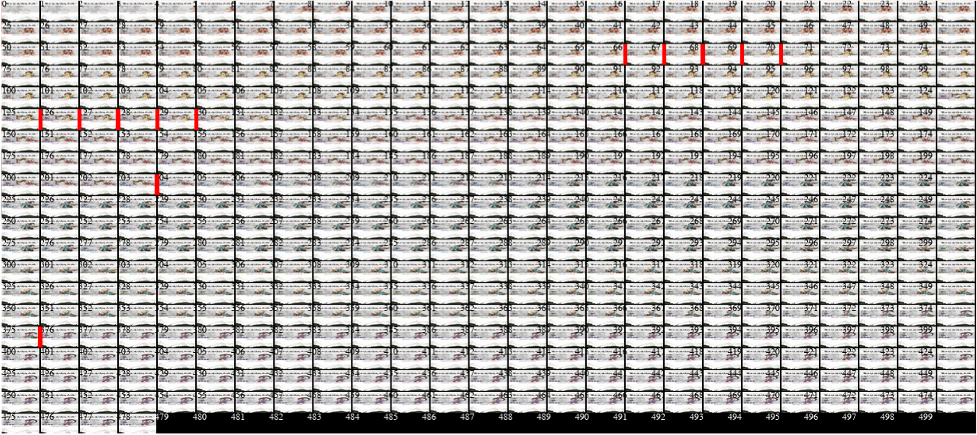}
  (d)
  \includegraphics[width=0.95\linewidth]{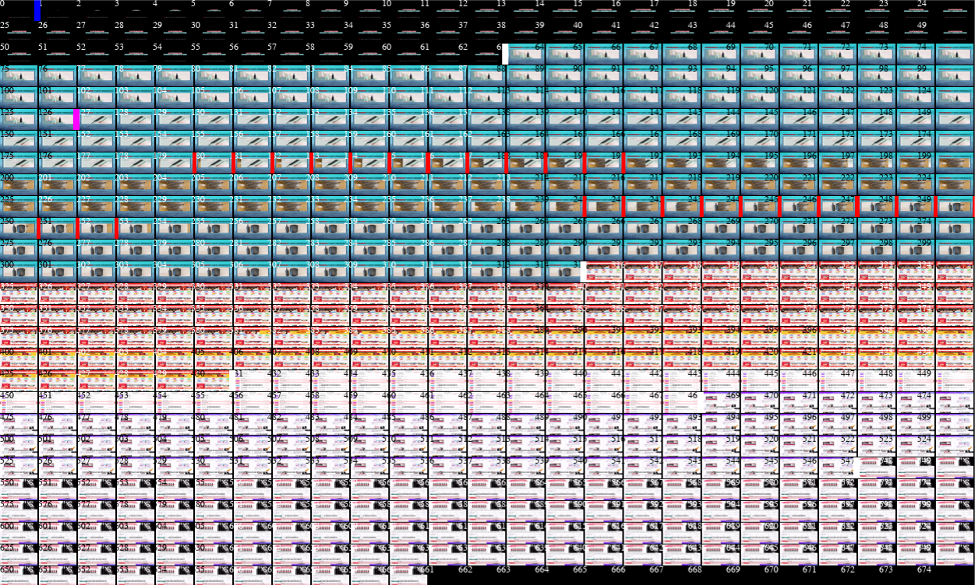}
   \caption{Visual comparison of shot boundaries of ground truth (red, light, pink, yellow), TransNetV2 (green, yellow, light, cyan), and AutoShot (blue, pink, light, cyan) on the collected SHOT dataset. AutoShot detects minor transition, shown in the pink color. The light color denotes that both the TransNetV2 and AutoShot successfully detects the shot boundary.}  % The video thumbnail image clearly demonstrates shot transitions, which greatly reduces the annotation labor and is a useful tool for high quality shot boundary annotation.
   \label{fig:pred_supp}
\end{figure}

{\small
\bibliographystyle{ieee_fullname}
\bibliography{egbib}
}

\end{document}
